# Supplementary material for: Enabling Pareto-Stationarity Exploration in Multi-Objective Reinforcement Learning: A Multi-Objective Weighted-Chebyshev Actor-Critic Approach
Source: arXiv:2507.21397 source file (2025-07-29)
Supplement: Supplementary file 1 [file appendix.tex]

\section{Supporting Definitions, Lemmas and Critic Results}
\subsection{Definitions and Additional Assumptions}
Here, we first define some standard terms and reiterate Assumption 2 for clarity.

For each objective $i\in [M]$, we define the state-action value function as follows:
(i) for average total reward:
$Q^{i}_{\bm{\theta}}(s,a):=\mathbb{E}\left[\sum_{t=0}^\infty r^{i}(s_t,a_t)-J^i(\bm{\theta})|s_0=s,a_0=a\right]$, 
and (ii) for discounted total reward:
$Q^{i}_{\bm{\theta}}(s,a)=\mathbb{E}\left[\sum_{t=0}^{\infty}(\gamma^i)^t r^{i}(s_t,a_t)|s_0=s,a_0=a\right]$.
It then follows that the value function satisfies:
$V^{i}_{\bm{\theta}}(s)=\sum_{a\in\mathcal{A}}Q^{i}_{\bm{\theta}}(s,a)\cdot\pi_{\bm{\theta}}(a|s).$
We define the advantage function as follows: 
$\text{Adv}^{i}_{\bm{\theta}}(s,a)=Q^{i}_{\bm{\theta}}(s,a)-V^{i}_{\bm{\theta}}(s)$, $\forall i\in [M]$. %\label{eq: adv_fun}
% \end{equation*}

\begin{assumption}[Reiteration of Assumption \ref{ass:feature}]
    The value function of each objective $i$ is approximated by a linear function: $V^i(s) \approx \bm{\phi}(s)^{\top}\w^i, i\in[M]$, where $\w^i\in\mathbb{R}^{d_2}$ with $d_2\leq|\mathcal{S}|$ is a parameter to be learnt, and $\bm{\phi}(s)\in\mathbb{R}^{d_2}$ is the feature associated with state $s\in\mathcal{S}$, which satisfies:
    \begin{list}{\labelitemi}{\leftmargin=1.8em \itemindent=-1.2em \itemsep=-.2em}
    \item[(a)] All features are normalized, i.e., $\|\bm{\phi}(s)\|_2\leq 1, \forall s\in\mathcal{S}$;
    \item[(b)] The feature matrix $\Phi\in\mathbb{R}^{|\mathcal{S}|\times d_2}$ is full rank;
    \item[(c)] For any $u\in \mathbb{R}^{d_2}$, $\Phi u\neq \mathbf{1}$, where $\mathbf{1}\in\mathbb{R}^{d_2}$;
    \item[(d)] Let $\A_{\bm{\theta}}:=\mathbb{E}_{s\sim d_{\bm{\theta}}(\cdot), s'\sim P(\cdot|s)}[(\bm{\phi}(s')-\bm{\phi}(s))\bm{\phi}^{\top}(s)]$ if in average reward setting. Otherwise, if in discounted reward setting, let $\A_{\bm{\theta}}:=\mathbb{E}_{s\sim d_{\theta}(\cdot), s'\sim P(\cdot|s)}\left[\left(\gamma\bm{\phi}(s')-\bm{\phi}(s)\right)\bm{\phi}^{\top}(s)\right]$. Then, there exists a constant $\lambda_{\A}>0$ such that $\lambda_{\max}(\A_{\bm{\theta}}+\A^{\top}_{\bm{\theta}})\le -\lambda_{\A}$ for all $\theta\in \mathcal{R}^{d_1}$, where $\lambda_{\max}(\A)$ is the largest eigenvalue of the matrix $\A$. 
    \end{list}
    \vspace{-1em}
\label{ass:feature_full}
\end{assumption}
Assumption \ref{ass:feature} item (c) and item (d), which are used for average reward setting, imply that for any policy $\pi_{\bm{\theta}}$, the inequality $\w^{\top}\A_{\bm{\theta}}\w<0$ holds for any $\w\neq 0$, and $\A_{\pi_{\bm{\theta}}}$ is invertible with $\lambda_{\max}(\A_{\bm{\theta}}+\A^{\top}_{\bm{\theta}})\le 0$.
This ensures that the optimal approximation $\w^{i,*}_{\bm{\theta}}$ for any given policy $\pi_{\bm{\theta}}$ and $i\in [M]$ is uniformly bounded.
Assumption~\ref{ass:feature_full} has been widely use in the literature (e.g., \cite{TsiVan_99,ZhaYanLiu_18,QiuYanYe_21}).

\subsection{Supporting Lemmas}
The following lemma characterizes the mixing time of the underlying Markov chain and the data sampled in \policy follows such Markovian chain, which holds under Assumption~\ref{ass:mdp} \cite[Theorem~4.9]{levin2017markov}.
\begin{lemma} \label{lem:mixing}
For any policy $\pi_{\bm{\theta}}$, consider an MDP with $P(\cdot\mid s,a)$ and stationary distribution $d_{\bm{\theta}}(\cdot)$. 
There exist constants $\kappa>0$ and $\rho\in(0, 1)$ such that
$\sup_{s\in\mathcal{S}}\| P(s_t\mid s_0=s)-d_{\bm{\theta}}(\cdot) \|_{TV}\leq \kappa\rho^t.$ 
\end{lemma}

\begin{lemma}[Average reward setting]
Given a policy $\pi_{\bm{\theta}}$, for any objective $i\in[M]$, the TD fixed point for average reward setting $\w_{\bm{\theta}}^{i,*}$ is uniformly bounded, specifically, there exists constant $R_{\w}=4r_{\max}/\lambda_A>0$ such that
\begin{equation*}
    \|\w_{\bm{\theta}}^{i,*}\|\leq R_{\w}, \forall i\in[M].
\end{equation*}
\end{lemma}
\begin{proof}
\begin{align*}
\|\w^{i,*}_{\bm{\theta}}\|_2
&= \|-A_{\pi_{\bm{\theta}}}^{-1}\b^i_{\pi_{\bm{\theta}}}\|_2\\
&= \| -\mathbb{E}_{s\sim d_{\bm{\theta}}(s), s'\sim P(\cdot|s)}[(\bm{\phi}(s')-\bm{\phi}(s))\bm{\phi}^{T}(s)]^{-1}\cdot \mathbb{E}_{s\sim d_{\bm{\theta}},a\sim\pi_{\bm{\theta}}}\left[\bm{\phi}(s)\left(r^i(s,a)-J^i(\bm{\theta})\right)\right] \|_2\\
&\leq \| -\mathbb{E}_{s\sim d_{\bm{\theta}}(s), s'\sim P(\cdot|s)}[(\bm{\phi}(s')-\bm{\phi}(s))\bm{\phi}^{T}(s)]^{-1}\|_2\cdot \|\mathbb{E}_{s\sim d_{\bm{\theta}},a\sim\pi_{\bm{\theta}}}\left[\bm{\phi}(s)\left(r^i(s,a)-J^i(\bm{\theta})\right)\right] \|_2\\
&\overset{\text{(i)}}{=} \cfrac{\|\mathbb{E}_{s\sim d_{\bm{\theta}},a\sim\pi_{\bm{\theta}}}\left[\bm{\phi}(s)\left(r^i(s,a)-J^i(\bm{\theta})\right)\right] \|_2}{{\sigma_{\min}}\left( \| -\mathbb{E}_{s\sim d_{\bm{\theta}}(s), s'\sim P(\cdot|s)}[(\bm{\phi}(s')-\bm{\phi}(s))\bm{\phi}^{T}(s)]\|_2 \right)}\\
&\overset{\text{(ii)}}{\leq} \cfrac{2\|\mathbb{E}_{s\sim d_{\bm{\theta}},a\sim\pi_{\bm{\theta}}}\left[\bm{\phi}(s)\left(r^i(s,a)-J^i(\bm{\theta})\right)\right] \|_2}{\lambda_A\left( -A_{\pi_{\bm{\theta}}} -A_{\pi_{\bm{\theta}}}^\top \right)}\\
&\leq \cfrac{2\cdot\mathbb{E}_{s\sim d_{\bm{\theta}},a\sim\pi_{\bm{\theta}}}\left[\|\bm{\phi}(s)\|_2\cdot \left(|r^i(s,a)|+|J^i(\bm{\theta})|\right)\right] }{\lambda_A}\\
&= \cfrac{4r_{\max}}{\lambda_A},
\end{align*}
where (i) follows from the fact $\|A^{-1}\|=1/\sigma_{\min}(A)$, and (ii) follows from \cite{bhatia2013matrix} (Proposition III 5.1).
\end{proof}

\begin{lemma}[Discounted reward setting]
Given a policy $\pi_{\bm{\theta}}$, for any objective $i\in[M]$, the value function approximation parameter $\w_{\bm{\theta}}^{i,*}$ is uniformly bounded, specifically, there exists constant $R_{\w}=2r_{\max}/\lambda_A>0$ such that
\begin{equation*}
    \|\w_{\bm{\theta}}^{i,*}\|\leq R_{\w}, \forall i\in[M].
\end{equation*}
\end{lemma}
\begin{proof}
\begin{align*}
\|\w^{i,*}_{\bm{\theta}}\|_2
&= \|-A_{\pi_{\bm{\theta}}}^{-1}\b^i_{\pi_{\bm{\theta}}}\|_2\\
&= \| -\mathbb{E}_{s\sim d_{\bm{\theta}}(s), s'\sim P(\cdot|s)}\left[\left(\gamma\bm{\phi}(s')-\bm{\phi}(s)\right)\bm{\phi}^{T}(s)\right]^{-1}\cdot \mathbb{E}_{s\sim d_{\bm{\theta}},a\sim\pi_{\bm{\theta}}}\left[r^i(s,a)\bm{\phi}(s)\right] \|_2\\
&\leq \| -\mathbb{E}_{s\sim d_{\bm{\theta}}(s), s'\sim P(\cdot|s)}\left[\left(\gamma\bm{\phi}(s')-\bm{\phi}(s)\right)\bm{\phi}^{T}(s)\right]^{-1}\|_2\cdot \|\mathbb{E}_{s\sim d_{\bm{\theta}},a\sim\pi_{\bm{\theta}}}\left[r^i(s,a)\bm{\phi}(s)\right] \|_2\\
&= \cfrac{\|\mathbb{E}_{s\sim d_{\bm{\theta}},a\sim\pi_{\bm{\theta}}}\left[r^i(s,a)\bm{\phi}(s)\right] \|_2}{\| -\mathbb{E}_{s\sim d_{\bm{\theta}}(s), s'\sim P(\cdot|s)}\left[\left(\gamma\bm{\phi}(s')-\bm{\phi}(s)\right)\bm{\phi}^{T}(s)\right]\|_2}\\
&\leq \cfrac{2\|\mathbb{E}_{s\sim d_{\bm{\theta}},a\sim\pi_{\bm{\theta}}}\left[r^i(s,a)\bm{\phi}(s)\right] \|_2}{\lambda_A\left( -A_{\pi_{\bm{\theta}}} -A_{\pi_{\bm{\theta}}}^\top \right)}\\
&\leq \cfrac{2\cdot\mathbb{E}_{s\sim d_{\bm{\theta}},a\sim\pi_{\bm{\theta}}}\left[\|\bm{\phi}(s)\|_2\cdot |r^i(s,a)|\right] }{\lambda_A}\\
&= \cfrac{2r_{\max}}{\lambda_A}.
\end{align*}
\end{proof}

\begin{lemma}(\cite{HaiLiuLu_22} Lemma~2)
Let $\nu_{\bm{\theta}}$ denote the stationary distribution of the state-action pairs given policy $\pi_{\bm{\theta}}$, there exists constants $\kappa>0$ and $\rho\in(0, 1)$ such that
\begin{equation*}
    \sup_{s\in\mathcal{S}}\| P(s_t, a_t\mid s_0=s)-\nu_{\bm{\theta}} \|_{TV}\leq \kappa\rho^t.
\end{equation*}
\label{lemma:tv2}
\end{lemma}

\begin{lemma}(\cite{HaiLiuLu_22} Lemma~3)
Suppose Assumption~\ref{ass:feature} holds. Given a policy $\pi_{\bm{\theta}}$, we have the following:
\begin{equation*}
(-\w^{i,*}_{\bm{\theta}})^{\top} \A_{\pi_{\bm{\theta}}}(-\w^{i,*}_{\bm{\theta}})\le -\frac{\lambda_{\A}}{2}\|\w^{i,*}_{\bm{\theta}}\|^{2}_2.
\end{equation*}
\end{lemma}

\begin{lemma}(\cite{XuWanLia_20} Theorem~4)
For any $i\in[M]$, consider mini-batch linear stochastic approximation on $\A_{\pi_{\bm{\theta}}}$, $\b_{\bm{\theta}}'^i$ (discounted setting), and $\b_{\bm{\theta}}^i$ (average setting). Let $C_{\A}>\|\A_{\pi_{\bm{\theta}}}\|_F$ and $C_{\b}$ denote the upper bound for $\|\b_{\bm{\theta}}^i\|_2$ and $\|\b_{\bm{\theta}}'^i\|_2$, then by setting $\beta\leq \min\lbrace {\lambda_{\A}\over 8C_{\A}^2}, {4\over\lambda_{\A}}\rbrace$ and $D\geq \left({2\over\lambda_{\A}}+2\beta\right){192C_{\A}^2[1+\rho(\kappa-1)]\over(1-\rho)\lambda_{\A}}$ and we have
\begin{equation*}
\mathbb{E}\big[ \| \w^i_N - \w^{i,*}_{\bm{\theta}} \|^2_2 \big] \leq \left( 1 - \cfrac{\beta\lambda_{\A}}{8} \right)^N \cdot\| \w^{i}_0 - \w^{i,*}_{\bm{\theta}} \|^2_2 + \left({2\over\lambda_{\A}}+2\beta\right){192\left(C_{\A}^2R_{\w}^2+C_{\b}^2\right)[1+\rho(\kappa-1)]\over(1-\rho)\lambda_{\A}D}.
\end{equation*}
Further, setting $N\geq{8\over\beta\lambda_{\A}}\log\left(2\| \w^{i}_0 - \w^{i,*}_{\bm{\theta}} \|^2_2/\epsilon\right)$ and $D\geq \left({2\over\lambda_{\A}}+2\beta\right){192\left(C_{\A}^2R_{\w}^2+C_{\b}^2\right)[1+\rho(\kappa-1)]\over\epsilon(1-\rho)\lambda_{\A}}$, we have $\mathbb{E}\big[ \| \w^i_N - \w^{i,*}_{\bm{\theta}} \|^2_2 \big]\leq\epsilon$ with total sample complexity $ND = \mathcal{O}\left(\epsilon^{-1}\log{(\epsilon^{-1})}\right)$.
\label{lemma:xu}
\end{lemma}

\subsection{Theoretical Results of the Critic of \policyns} \label{sec:critic}
The critic component of \policy outputs $M$ value function approximation parameters based on the same sequences of Markovian samplings.
In the average reward setting, given a policy parameter $\bm{\theta}$, define vector $\b^i_{\bm{\theta}}:=\mathbb{E}_{s\sim d_{\bm{\theta}},a\sim\pi_{\bm{\theta}}}\left[\left(r^i(s,a)-J^i(\bm{\theta})\right)\bm{\phi}(s)\right], \forall i\in[M]$.
Then the fixed point of TD-learning for objective $i$ is $\w^{i,*}_{\bm{\theta}}=-\A_{\pi_{\bm{\theta}}}^{-1}\b^i_{\bm{\theta}}$, where $\A_{\pi_{\bm{\theta}}}$ is defined in Assumption~\ref{ass:feature}(d).
Similarly, in the discounted reward setting, define vector $\b'^i_{\bm{\theta}}:=\mathbb{E}_{s\sim d_{\bm{\theta}},a\sim\pi_{\bm{\theta}}}\left[r^i(s,a)\bm{\phi}(s)\right]$ and we have $\w^{i,*}_{\bm{\theta}}=-\A^{-1}_{\pi_{\bm{\theta}}}\b'^i_{\bm{\theta}}$, $\forall i\in[M]$. Let constant $C_{\A}>\|\A_{\pi_{\bm{\theta}}}\|_F$, where $\|\cdot\|_F$ denotes the Frobenius Norm.
We now state the convergence of the critic step of \policy as follows:
\begin{theorem}{\em
Under Assumptions \ref{ass:mdp}-\ref{ass:Lip_bou}, for both average and discounted settings, let the critic step size $\beta\leq \min\lbrace {\lambda_{\A}\over 8C_{\A}^2}, {4\over\lambda_{\A}}\rbrace$.
Then, for any objective $i\in[M]$, the iterations generated by Algorithm~\ref{alg: pf-moac} satisfy the following finite-time convergence error bound:
\begin{equation}
    \mathbb{E}\big[ \| \w^i_N \!-\! \w^{i,*}_{\bm{\theta}} \|^2_2 \big] \!\leq\! C_1\big( 1\!-\!\cfrac{\beta\lambda_{\A}}{8} \big)^N \!\!+\! \cfrac{C_2C_3({2\over\lambda_{\A}}\!+\!2\beta)}{\lambda_{\A}D},\!\!
\label{eq:critic}
\end{equation}
where $C_1=\| \w^i_0 - \w^{i,*}_{\bm{\theta}} \|^2_2$, $C_2=[1+(\kappa-1)\rho]/(1-\rho)$, and $C_3>0$ is a constant depending on $\A_{\pi_{\bm{\theta}}}$, $\b_{\bm{\theta}}^i$, and $\b_{\bm{\theta}}'^i$.
}
\label{thm:critic}
\end{theorem}

\begin{proof}
The results of Theorem~\ref{thm:critic} follows directly from Lemma~\ref{lemma:xu}, by setting $\A_{\pi_{\bm{\theta}}}:=\mathbb{E}_{s\sim d_{\bm{\theta}}(s), s'\sim P(\cdot|s)}[(\bm{\phi}(s')-\bm{\phi}(s))\bm{\phi}^{\top}(s)]$ and $\b^i_{\bm{\theta}}:=\mathbb{E}_{s\sim d_{\bm{\theta}},a\sim\pi_{\bm{\theta}}}\left[\left(r^i(s,a)-J^i(\bm{\theta})\right)\bm{\phi}(s)\right], \forall i\in[M]$ for the average reward setting, and by setting $\A_{\pi_{\theta}}:=\mathbb{E}_{s\sim d_{\theta}(s), s'\sim P(\cdot|s)}\left[\left(\gamma\bm{\phi}(s')-\bm{\phi}(s)\right)\bm{\phi}^{T}(s)\right]$ and $\b'^i_{\bm{\theta}}:=\mathbb{E}_{s\sim d_{\bm{\theta}},a\sim\pi_{\bm{\theta}}}\left[r^i(s,a)\bm{\phi}(s)\right], \forall i\in[M]$ for the discounted reward setting.

For clarity, we present Theorem~\ref{thm:critic} with some terms simplified as constants, where $C_1=\| \w^i_0 - \w^{i,*}_{\bm{\theta}} \|^2_2$, $C_2=[1+(\kappa-1)\rho]/(1-\rho)$, and $C_3=192\left(C_{\A}^2R_{\w}^2+C_{\b}^2\right)$.
\end{proof}

Theorem \ref{thm:critic} states that critic component of Algorithm~\ref{alg: pf-moac} will evaluate and maintain a value function parameter $w^{i}_{\bm{\theta}}$ each objective $i\in [M]$ for the given policy $\pi_{\bm{\theta}}$. Compared to many existing works \cite{LakSze_18,doan2018distributed,ZhaLiuLiu_21} in RL algorithm finite-time convergence analysis, the samples in our method are correlated (i.e., Markovian noise) instead of i.i.d. noise, which is equivalent to $\rho=0$. 
Despite the fact that Markovian noise introduces extra bias error seen from term $C_2$, our batching approach with size $D>1$ offer two-fold benefits: 
1) Part of the convergence error can be controlled with increasing $D$ (cf. the second term on the RHS in Eq.~(\ref{eq:critic}); 
2) it allows the use of {\em constant} step size, leading to a better sample complexity comparing to non-batch approach \cite{srikant2019finite,QiuYanYe_21,HaiZhaLiu_24} and faster convergence in practice in general.

Theorem~\ref{thm:critic} immediately implies the following sample complexity results for the critic component in \policyns:

\begin{corollary}
For both average and discounted settings, let $N\geq{8\over\beta\lambda_{\A}}\log(2C_1/\epsilon)$ and $D\geq C_2C_3\big( {2\over\lambda_{\A}}+2\beta \big)/(\epsilon\lambda_{\A})$.
It then holds that $\mathbb{E}\big[ \| \w^i_N - \w^{i,*}_{\bm{\theta}} \|^2_2 \big]\leq\epsilon, i\in[M]$, which implies a sample complexity of $\mathcal{O}(\epsilon^{-1}\log(\epsilon^{-1}))$.
\label{coro:critic}
\end{corollary}

\section{Proof of Theorem~\ref{thm:moac1}}
We first present the proof in average reward setting, then we show how to obtain the results in discounted reward setting.
\begin{proof}
For any given $\bm{\theta}$ and its associated policy $\pi_{\bm{\theta}}$, we denote the gradient matrix to be
\begin{align}
\nabla_{\bm{\theta}}\J(\bm{\theta})=
\left[\begin{matrix}
\nabla_{\bm{\theta}} J^{1}(\bm{\theta}) &
\nabla_{\bm{\theta}} J^{2}(\bm{\theta}) &
\cdots &
\nabla_{\bm{\theta}} J^{M}(\bm{\theta})
\end{matrix}\right] \in \mathbb{R}^{d_1\times M}.  \nonumber
\end{align}
Given $\bm{\theta}\in\mathbb{R}^{d_1}$, $\w\in\mathbb{R}^{d_2}$, for $t\geq 0$ and for any $i\in [M]$, by Lipschitzness in Assumption \ref{ass:Lip_bou},
we have
\begin{align}
J^{i}(\bm{\theta}_{t+1})\ge J^{i}(\bm{\theta}_t)+\left\langle \nabla_{\bm{\theta}}J^{i}(\bm{\theta}_t), \bm{\theta}_{t+1} - \bm{\theta}_t \right\rangle - \cfrac{L_J}{2}\|\bm{\theta}_{t+1} - \bm{\theta}_t\|^2. \label{eq: j_gra_i}
\end{align}
Note that $J^{i}(\bm{\theta})$ is an expected value taken, where the expectation is taken over steady-state distribution induced by policy $\pi_{\bm{\theta}}$. We use $\bm{\lambda}^{*}_t$ to denote solution for $\bm{\lambda}\geq \bm{0}$, $\1^{\top}\bm{\lambda}=1$, such that $\min_{\bm{\lambda}}\|\nabla_{\bm{\theta}}\J(\bm{\theta}_t)\bm{\lambda}\|_2$. In comparison, $\bm{\lambda}_t$ is the QP solution with momentum in Equation \eqref{eq:lambda} for using $\{\g_t^i\}_{i\in [M]}$ as in Algorithm \ref{alg: pf-moac}. 

Let $\bm{q}_t:=\frac{\bm{\lambda}_t\odot \p}{\langle \bm{\lambda}_t,\p\rangle}$, $l_t:=\langle \bm{\lambda}_t,\p\rangle$ and $p_{\min}:=\min_{i\in[M]} \p_i$. Note that $p_{\min}\le l_t\le 1$. For $t>0$, $\bm{q}_t$ serves as a pseudo-weight for the actor convergence analysis and $l_t$ measures the length of it.

Taking $\bm{q}_t$ weighted summation over Eq. \eqref{eq: j_gra_i}, we have
\begin{align}
    \bm{q}_t^{\top} \bm{J}(\bm{\theta}_{t+1})&\geq \bm{q}_t^\top\bm{J}(\bm{\theta}_t) + \left\langle \nabla_{\bm{\theta}}\bm{J}(\bm{\theta}_t)\bm{q}_t, \bm{\theta}_{t+1} - \bm{\theta}_t \right\rangle - \cfrac{L_J}{2}\|\bm{\theta}_{t+1} - \bm{\theta}_t\|_2^2\nonumber\\
    &= \bm{q}_t^\top\bm{J}(\bm{\theta}_t) + \alpha l_t\left\langle \nabla_{\bm{\theta}}\bm{J}(\bm{\theta}_t)\bm{q}_t, \sum_{j=1}^M q_t^{j}\g_t^j \right\rangle - \cfrac{\alpha^2L_J}{2}\|\g_t\|_2^2\nonumber\\
    &= \bm{q}_t^\top\bm{J}(\bm{\theta}_t) + \alpha l_t\left\langle \nabla_{\bm{\theta}}\bm{J}(\bm{\theta}_t)\bm{q}_t, \sum_{j=1}^M q_t^j\cdot\left(\g_t^j - \nabla_{\bm{\theta}}J^j(\bm{\theta}_t) + \nabla_{\bm{\theta}}J^j(\bm{\theta}_t)\right) \right\rangle - \cfrac{\alpha^2L_J}{2}\|\g_t\|_2^2\nonumber\\
    &= \bm{q}_t^\top\bm{J}(\bm{\theta}_t) + \alpha l_t\left\langle \nabla_{\bm{\theta}}\bm{J}(\bm{\theta}_t)\bm{q}_t, \sum_{j=1}^M q_t^j\nabla_{\bm{\theta}}J^j(\bm{\theta}_t) \right\rangle\nonumber\\
    &\hspace{13pt} + \alpha l_t\left\langle \nabla_{\bm{\theta}}\bm{J}(\bm{\theta}_t)\bm{q}_t, \sum_{j=1}^M q_t^j\cdot\left(\g_t^j - \nabla_{\bm{\theta}}J^j(\bm{\theta}_t)\right) \right\rangle- \cfrac{\alpha^2L_J}{2}\|\g_t\|_2^2\nonumber\\
    &= \bm{q}_t^\top\bm{J}(\bm{\theta}_t) + \alpha l_t\left\|\nabla_{\bm{\theta}}\bm{J}(\bm{\theta}_t)\bm{q}_t\right\|^2_2 + \alpha l_t\left\langle \nabla_{\bm{\theta}}\bm{J}(\bm{\theta}_t)\bm{q}_t, \sum_{j=1}^M q_t^j\cdot\left(\g_t^j - \nabla_{\bm{\theta}}J^j(\bm{\theta}_t)\right) \right\rangle - \cfrac{\alpha^2L_J}{2}\|\g_t\|_2^2\nonumber\\
    &\overset{\text{(i)}}{\geq} \bm{q}_t^\top\bm{J}(\bm{\theta}_t) + \cfrac{\alpha l_t}{2}\left\|\nabla_{\bm{\theta}}\bm{J}(\bm{\theta}_t)\bm{q}_t\right\|^2_2 - \cfrac{\alpha l_t}{2}\left\|\sum_{j=1}^M q_t^j\cdot\left(\nabla_{\bm{\theta}}J^j(\bm{\theta}_t)-\g_t^j\right) \right\|^2_2 - \cfrac{\alpha^2L_J}{2}\|\g_t\|_2^2\nonumber\\
    &= \bm{q}_t^\top\bm{J}(\bm{\theta}_t) + \cfrac{\alpha l_t}{2}\left\|\nabla_{\bm{\theta}}\bm{J}(\bm{\theta}_t)\bm{q}_t\right\|^2_2 - \cfrac{\alpha l_t}{2}\left\|\sum_{j=1}^M q_t^j\cdot\left(\nabla_{\bm{\theta}}J^j(\bm{\theta}_t)-\g_t^j\right) \right\|^2_2\nonumber\\
    &\hspace{13pt}- \cfrac{\alpha^2 l^{2}_t L_J}{2}\left\|\sum_{j=1}^M q_t^j\cdot\left(\g_t^j - \nabla_{\bm{\theta}}J^j(\bm{\theta}_t) + \nabla_{\bm{\theta}}J^j(\bm{\theta}_t)\right)\right\|_2^2\nonumber\\
    &\overset{\text{(ii)}}{\geq} \bm{q}_t^\top\bm{J}(\bm{\theta}_t) + \left(\cfrac{\alpha l_t}{2}-\alpha^2 l^{2}_t L_J\right)\left\|\nabla_{\bm{\theta}}\bm{J}(\bm{\theta}_t)\bm{q}_t\right\|^2_2 - \left(\cfrac{\alpha l_t}{2}+\alpha^2 l^{2}_t L_J\right)\left\|\sum_{j=1}^M q_t^j\cdot\left(\nabla_{\bm{\theta}}J^j(\bm{\theta}_t)-\g_t^j\right) \right\|^2_2,
\label{eq:2}
\end{align}
where inequality (i) follows from
\begin{equation*}
    \left\langle \nabla_{\bm{\theta}}\bm{J}(\bm{\theta}_t)\bm{q}_t, \sum_{j=1}^M q_t^j\cdot\left(\g_t^j-\nabla_{\bm{\theta}}J^j(\bm{\theta}_t)\right) \right\rangle\geq -\cfrac{1}{2}\left\|\nabla_{\bm{\theta}}\bm{J}(\bm{\theta}_t)\bm{q}_t\right\|^2_2 - \cfrac{1}{2}\left\|\sum_{j=1}^M q_t^j\cdot\left(\nabla_{\bm{\theta}}J^j(\bm{\theta}_t)-\g_t^j\right) \right\|^2_2,
\end{equation*}
and inequality (ii) follows from
\begin{equation*}
    \left\|\sum_{j=1}^M q_t^j\cdot\left(\g_t^j - \nabla_{\bm{\theta}}J^j(\bm{\theta}_t) + \nabla_{\bm{\theta}}J^j(\bm{\theta}_t)\right)\right\|_2^2\leq 2\left\|\nabla_{\bm{\theta}}\bm{J}(\bm{\theta}_t)\bm{q}_t\right\|^2_2 + 2\left\|\sum_{j=1}^M q_t^j\cdot\left(\nabla_{\bm{\theta}}J^j(\bm{\theta}_t)-\g_t^j\right) \right\|^2_2.
\end{equation*}
Taking expectation on both sides of Eq.~(\ref{eq:2}) and conditioning on $\mathcal{F}_t$, we have
\begin{equation*}
    \mathbb{E}\left[ \left\|\nabla_{\bm{\theta}}\bm{J}(\bm{\theta}_t)\bm{q}_t\right\|^2_2 \mid \mathcal{F}_t \right] \leq \cfrac{2\left(\mathbb{E}\left[\bm{q}_t^\top\bm{J}(\bm{\theta}_{t+1})\vert \mathcal{F}_t\right] - \bm{q}_t^\top\bm{J}(\bm{\theta}_t)\right)}{\alpha l_t-2\alpha^2 l^{2}_t L_J} + \cfrac{\alpha+2\alpha^2 l_t L_J}{\alpha-2\alpha^2 l_t L_J}\mathbb{E}\left[\left\|\sum_{j=1}^M q_t^j\left(\nabla_{\bm{\theta}}J^j(\bm{\theta}_t)-\g_t^j\right) \right\|^2_2\bigg\vert \mathcal{F}_t\right].
\end{equation*}
By the definitions of $\bm{\lambda}^*_t$ and $\bm{q}_t$, for any time $t$, we have
\begin{equation*}
    \mathbb{E}\left[ \left\|\nabla_{\bm{\theta}}\bm{J}(\bm{\theta}_t)\bm{\lambda}_t^*\right\|^2_2 \mid \mathcal{F}_t \right] \leq \mathbb{E}\left[ \left\|\nabla_{\bm{\theta}}\bm{J}(\bm{\theta}_t)\bm{q}_t\right\|^2_2 \mid \mathcal{F}_t \right].
\end{equation*}
Therefore, we have
\begin{equation}
    \mathbb{E}\left[ \left\|\nabla_{\bm{\theta}}\bm{J}(\bm{\theta}_t)\bm{\lambda}_t^*\right\|^2_2 \mid \mathcal{F}_t \right] \leq \cfrac{2\left(\mathbb{E}\left[\bm{q}_t^\top\bm{J}(\bm{\theta}_{t+1})\vert \mathcal{F}_t\right] - \bm{q}_t^\top\bm{J}(\bm{\theta}_t)\right)}{\alpha l_t-2\alpha^2 l^{2}_t L_J} + \cfrac{\alpha+2\alpha^2 l_t L_J}{\alpha-2\alpha^2 l_t L_J}\mathbb{E}\left[\left\|\sum_{j=1}^M q_t^j\left(\nabla_{\bm{\theta}}J^j(\bm{\theta}_t)-\g_t^j\right) \right\|^2_2\bigg\vert \mathcal{F}_t\right].
\label{eq: dir_mod}
\end{equation}

\subsection{For the 2nd Term on RHS of Eq.~\eqref{eq: dir_mod}}
Define a notation: $\Delta^j_{\bm{\theta}_t, \w_t^*}=\mathbb{E}_{d_{\bm{\theta}}}\left[\mathbb{E}_{P_{\bm{\theta}}}\left[\delta_{t,l}^j(\w_t^{j,*})\mid(a_{t,l},s_{t,l})\right]\cdot\bm{\psi}^{\bm{\theta}}_{t, l}\right]$.
We first bound the last term on the right hand side of Eq.~\eqref{eq: dir_mod} as follows:
\begin{align}
    &\hspace{13pt}\mathbb{E}\left[\left\|\sum_{j=1}^M \lambda_t^j\left(\nabla_{\bm{\theta}}J^j(\bm{\theta}_t)-\g_t^j\right) \right\|^2_2\bigg\vert \mathcal{F}_t\right]\nonumber\\
    &\leq \mathbb{E}\left[\left(\sum_{j=1}^M \lambda_t^j\left\|\nabla_{\bm{\theta}}J^j(\bm{\theta}_t)-\g_t^j\right\|_2
    \right)^2\bigg\vert \mathcal{F}_t\right]\nonumber\\
    &\leq \mathbb{E}\left[ \left(\sum_{j=1}^M \lambda_t^j \left(\left\| \nabla_{\bm{\theta}}J^j(\bm{\theta}_t) - \Delta^j_{\bm{\theta}_t,\w_t^*}\right\|_2 + \left\| \Delta^j_{\bm{\theta}_t,\w_t^*} -\g^j_{\bm{\theta}_t^*}\right\|_2 + \left\| \g^j_{\bm{\theta}_t^*} - \g_t^j\right\|_2\right) \right)^2 \bigg\vert \mathcal{F}_t \right]\nonumber\\
    &\le 3\mathbb{E}\left[\left(\sum_{j=1}^M \lambda_t^j \left\| \nabla_{\bm{\theta}}J^j(\bm{\theta}_t) - \Delta^j_{\bm{\theta}_t,\w_t^*}\right\|_2  \right)^2\bigg\vert \mathcal{F}_t \right]+ 3\mathbb{E}\left[\left(\sum_{j=1}^M \lambda_t^j \left\| \g^j_{\bm{\theta}_t^*} - \g_t^j\right\|_2 \right)^{2}\bigg\vert  \mathcal{F}_t \right]\nonumber\\
    &\hspace{13pt}+ 3\mathbb{E}\left[ \left(\sum_{j=1}^M \lambda_t^j \cdot\left\| \Delta^j_{\bm{\theta}_t,\w_t^*} -\g^j_{\bm{\theta}_t^*}\right\|_2 \right)^2 \bigg\vert \mathcal{F}_t \right], \label{eq:4} 
    %&\le 2\mathbb{E}\left[ \left(\sum_{j=1}^M \lambda_t^j \left(\left\| \nabla_{\bm{\theta}}J^j(\bm{\theta}_t) - \Delta^j_{\bm{\theta}_t,\w_t^*}\right\|_2 + \left\| \g^j_{\bm{\theta}_t^*} - \g_t^j\right\|_2 \right) \right)^2 \bigg\vert \mathcal{F}_t \right] + 2\mathbb{E}\left[ \left(\sum_{j=1}^M \lambda_t^j \cdot\left\| \Delta^j_{\bm{\theta}_t,\w_t^*} -\g^j_{\bm{\theta}_t^*}\right\|_2 \right)^2 \bigg\vert \mathcal{F}_t \right]\label{eq:4},
\end{align}
where
\begin{align}
    \left\| \nabla_{\bm{\theta}}J^j(\bm{\theta}_t) - \Delta^j_{\bm{\theta}_t,\w_t^*}\right\|^{2}_2&=\left\|\mathbb{E}_{d_{\bm{\theta}}}\left[\mathbb{E}_{P_{\bm{\theta}}}\left[\delta_{t,l}^j\mid(a_{t,l},s_{t,l})\right]\cdot\bm{\psi}^{\bm{\theta}}_{t, l}\right] - \mathbb{E}_{d_{\bm{\theta}}}\left[\mathbb{E}_{P_{\bm{\theta}}}\left[\delta_{t,l}^j(\w_t^{j,*})\mid(a_{t,l},s_{t,l})\right]\cdot\bm{\psi}^{\bm{\theta}}_{t, l}\right]\right\|^{2}_2\nonumber\\
    &= \left\|\mathbb{E}_{d_{\bm{\theta}}}\left[\left(\mathbb{E}_{P_{\bm{\theta}}}\left[\delta_{t,l}^j\mid(a_{t,l},s_{t,l})\right] - \mathbb{E}_{P_{\bm{\theta}}}\left[\delta_{t,l}^j(\w_t^{j,*})\mid(a_{t,l},s_{t,l})\right]\right)\cdot\bm{\psi}^{\bm{\theta}}_{t, l}\right]\right\|^{2}_2\nonumber\\
    &\leq \mathbb{E}_{d_{\bm{\theta}}}\left[\left\|\left(\mathbb{E}_{P_{\bm{\theta}}}\left[\delta_{t,l}^j\mid(a_{t,l},s_{t,l})\right] - \mathbb{E}_{P_{\bm{\theta}}}\left[\delta_{t,l}^j(\w_t^{j,*})\mid(a_{t,l},s_{t,l})\right]\right)\cdot\bm{\psi}^{\bm{\theta}}_{t, l}\right\|^{2}_2\right]\nonumber\\
    &\leq \mathbb{E}_{d_{\bm{\theta}}}\left[\left|\mathbb{E}_{P_{\bm{\theta}}}\left[\delta_{t,l}^j\mid(a_{t,l},s_{t,l})\right] - \mathbb{E}_{P_{\bm{\theta}}}\left[\delta_{t,l}^j(\w_t^{j,*})\mid(a_{t,l},s_{t,l})\right]\right|^{2}\right]\nonumber\\    &=\mathbb{E}_{d_{\bm{\theta}}}\left[\left|\mathbb{E}\left[ V_{\bm{\theta}}^j(s_{t,l+1}) - V_{\bm{\theta}}^j(s_{t,l+1};\w_t^{j,*})\mid(a_{t,l},s_{t,l}) \right] + V_{\bm{\theta}}^j(s_{t,l}) - V_{\bm{\theta}}^j(s_{t,l};\w_t^{j,*})\right|^{2}\right]\nonumber\\
    &\le4 \zeta_{\text{approx}}. \nonumber
\end{align}
We note that $\delta^{j}_{t,l}$ denotes the TD error for objective $j\in [M]$ using the ground truth value functions.
We also remark that the above inequality holds for all $j\in [M]$. As a result, for the first term on the RHS of Eq.~\eqref{eq:4}, we have
\begin{equation}
\mathbb{E}\left[\left(\sum_{j=1}^M \lambda_t^j \left\| \nabla_{\bm{\theta}}J^j(\bm{\theta}_t) - \Delta^j_{\bm{\theta}_t,\w_t^*}\right\|_2  \right)^2\bigg\vert \mathcal{F}_t \right] \nonumber \le \mathbb{E}\left[\left(\sum_{j=1}^M \lambda_t^j 2\sqrt{\zeta_{\text{approx}}} \right)^2\bigg\vert \mathcal{F}_t \right]= 4 \zeta_{\text{approx}} \label{eq:5}
\end{equation}

Furthermore, we have
\begin{align}
    \left\| \g^j_{\bm{\theta}_t^*} - \g_t^j\right\|_2
    &= \left\| \cfrac{1}{B}\sum_{l=0}^{B-1}\left(\delta_{t,l}^j(\w^j_t) - \delta_{t,l}^j(\w^{j,*}_t) \right)\cdot\bm{\psi}^{\bm{\theta}}_{t,l} \right\|_2\nonumber\\
    &=\left\| \cfrac{1}{B}\sum_{l=0}^{B-1}\left( \bm{\phi}(s_{t,l+1}) - \bm{\phi}(s_{t,l}) \right)^{\top}\left( \w^j_t - \w^{j,*}_t \right)\cdot\bm{\psi}^{\bm{\theta}}_{t,l} \right\|_2\nonumber\\
    &\leq \left\| \cfrac{1}{B}\sum_{l=0}^{B-1}\left( \bm{\phi}(s_{t,l+1}) - \bm{\phi}(s_{t,l}) \right)^{\top}\left( \w^j_t - \w^{j,*}_t \right) \right\|_2\nonumber\\
    &\leq \max_{l\in\lbrace 0, \ldots, B-1\rbrace}\left\| \left( \bm{\phi}(s_{t,l+1}) - \bm{\phi}(s_{t,l}) \right)^{\top}\left( \w^j_t - \w^{j,*}_t \right) \right\|_2\nonumber\\
    &\leq 2\cdot\left\| \w^j_t - \w^{j,*}_t \right\|_2. \nonumber
\end{align}
As a result, for the second term on the RHS of Eq.~\eqref{eq:4}, we have
\begin{equation}
\mathbb{E}\left[\left(\sum_{j=1}^M \lambda_t^j \left\| \g^j_{\bm{\theta}_t^*} - \g_t^j\right\|_2 \right)^{2}\bigg\vert  \mathcal{F}_t \right] \le \mathbb{E}\left[\left(\sum_{j=1}^M \lambda_t^j 2\left\| \w^{j}_t-\w^{j,*}_t\right\|_2 \right)^{2}\bigg\vert  \mathcal{F}_t \right] \le 4 \max_{i\in[M]}\mathbb{E} \left[\left\| \w^{i}_t-\w^{i,*}_t\right\|^{2}_2 \bigg\vert  \mathcal{F}_t \right].\label{eq:6}
\end{equation}
For the second inequality above, it holds because
\begin{align}
&\mathbb{E}\left[\left(\sum_{j=1}^M \lambda_t^j \left\| \w^{j}_t-\w^{j,*}_t\right\|_2 \right)^{2}\bigg\vert  \mathcal{F}_t \right] \nonumber \\
=&\mathbb{E}\left[\sum_{j=1}^M (\lambda_t^j)^{2} \left\| \w^{j}_t-\w^{j,*}_t\right\|^{2}_2 +2\sum_{i\neq j}\lambda_t^{i}\lambda_t^{j} \left\| \w^{i}_t-\w^{i,*}_t\right\|_2\cdot\left\| \w^{j}_t-\w^{j,*}_t\right\|_2\bigg\vert  \mathcal{F}_t \right] \nonumber \\
=&\sum_{j=1}^M (\lambda_t^j)^{2} \mathbb{E}\left[\left\| \w^{j}_t-\w^{j,*}_t\right\|^{2}_2\bigg\vert  \mathcal{F}_t\right]  +2\sum_{i\neq j}\lambda_t^{i}\lambda_t^{j}  \mathbb{E}\left[\left\| \w^{i}_t-\w^{i,*}_t\right\|_2\cdot\left\| \w^{j}_t-\w^{j,*}_t\right\|_2\bigg\vert  \mathcal{F}_t \right] \nonumber \\
=&\sum_{j=1}^M (\lambda_t^j)^{2} \mathbb{E}\left[\left\| \w^{j}_t-\w^{j,*}_t\right\|^{2}_2\bigg\vert  \mathcal{F}_t\right]  +2\sum_{i\neq j}\lambda_t^{i}\lambda_t^{j}  \mathbb{E}\left[\left\| \w^{i}_t-\w^{i,*}_t\right\|_2\bigg\vert  \mathcal{F}_t \right]\cdot \mathbb{E}\left[\left\| \w^{j}_t-\w^{j,*}_t\right\|_2\bigg\vert  \mathcal{F}_t \right] \nonumber \\
\le &\sum_{j=1}^M (\lambda_t^j)^{2} \mathbb{E}\left[\left\| \w^{j}_t-\w^{j,*}_t\right\|^{2}_2\bigg\vert  \mathcal{F}_t\right]  +2\sum_{i\neq j}\lambda_t^{i}\lambda_t^{j}  \sqrt{\mathbb{E}\left[\left\| \w^{i}_t-\w^{i,*}_t\right\|^{2}_2\bigg\vert  \mathcal{F}_t \right]}\cdot \sqrt{\mathbb{E}\left[\left\| \w^{j}_t-\w^{j,*}_t\right\|^{2}_2\bigg\vert  \mathcal{F}_t \right]} \nonumber \\
\le &\left(\sum_{j=1}^M (\lambda_t^j)^{2}+2\sum_{i\neq j}\lambda_t^{i}\lambda_t^{j}\right)\max_{i\in [M]}\mathbb{E}\left[\left\| \w^{i}_t-\w^{i,*}_t\right\|^{2}_2\bigg\vert  \mathcal{F}_t \right]\nonumber \\
= &(\sum_{j=1}^M \lambda_t^j)^{2}\max_{i\in [M]}\mathbb{E}\left[\left\| \w^{i}_t-\w^{i,*}_t\right\|^{2}_2\bigg\vert  \mathcal{F}_t \right]\nonumber \\
= &\max_{i\in [M]}\mathbb{E}\left[\left\| \w^{i}_t-\w^{i,*}_t\right\|^{2}_2\bigg\vert  \mathcal{F}_t \right],\nonumber
\end{align}
where the third equality is due to the conditional independence of objective $i$ and $j$ given filtration $\mathcal{F}_t$ and the first inequality is because of $(\mathbb{E}[X])^{2}\le \mathbb{E}[X^{2}]$ for a random variable $X$.
Similarly, for the last term in Eq.~(\ref{eq:4}), we have
\begin{equation*}
    \mathbb{E}\bigg[ \bigg(\sum_{j=1}^M \lambda_t^j \cdot\left\| \Delta^j_{\bm{\theta}_t,\w_t^*} -\g^j_{\bm{\theta}_t^*}\right\|_2 \bigg)^2 \bigg\vert \mathcal{F}_t \bigg]
    \le\max_{i\in[M]}\mathbb{E}\bigg[ \bigg(\sum_{j=1}^M \lambda_t^j \cdot\left\| \Delta^i_{\bm{\theta}_t,\w_t^*} -\g^i_{\bm{\theta}_t^*}\right\|_2 \bigg)^2 \bigg\vert \mathcal{F}_t \bigg]
    = \max_{i\in[M]}\mathbb{E}\left[\left\| \Delta^i_{\bm{\theta}_t,\w_t^*} -\g^i_{\bm{\theta}_t^*}\right\|^{2}_2 \bigg\vert \mathcal{F}_t \right].
\end{equation*}
\begin{comment}
\begin{align*}
    &\hspace{13pt}\mathbb{E}\left[ \left(\sum_{j=1}^M \lambda_t^j \cdot\left\| \Delta^j_{\bm{\theta}_t,\w_t^*} -\g^j_{\bm{\theta}_t^*}\right\|_2 \right)^2 \bigg\vert \mathcal{F}_t \right]\\
    &\leq \mathbb{E}\left[ \left(\sum_{j=1}^M \left\| \Delta^j_{\bm{\theta}_t,\w_t^*} -\g^j_{\bm{\theta}_t^*}\right\|_2 \right)^2 \bigg\vert \mathcal{F}_t \right]\\
    &= \mathbb{E}\left[ \sum_{j_1=1}^M\left\| \Delta^{j_1}_{\bm{\theta}_t,\w_t^*} -\g^{j_1}_{\bm{\theta}_t^*} \right\|_2\cdot \sum_{j_2=1}^M\left\| \Delta^{j_2}_{\bm{\theta}_t,\w_t^*} -\g^{j_2}_{\bm{\theta}_t^*} \right\|_2 \bigg\vert\mathcal{F}_t\right]\\
    &= \mathbb{E}\left[ \sum_{j_1=1}^M\sum_{j_2=1}^M \left\| \Delta^{j_1}_{\bm{\theta}_t,\w_t^*} -\g^{j_1}_{\bm{\theta}_t^*} \right\|_2\cdot \left\| \Delta^{j_2}_{\bm{\theta}_t,\w_t^*} -\g^{j_2}_{\bm{\theta}_t^*} \right\|_2 \bigg\vert\mathcal{F}_t\right]\\
    &= \mathbb{E}\left[ \sum_{j=1}^M \left\| \Delta^{j}_{\bm{\theta}_t,\w_t^*} -\g^{j}_{\bm{\theta}_t^*} \right\|_2^2 + \sum_{j_1\neq j_2}\left\| \Delta^{j_1}_{\bm{\theta}_t,\w_t^*} -\g^{j_1}_{\bm{\theta}_t^*} \right\|_2\cdot \left\| \Delta^{j_2}_{\bm{\theta}_t,\w_t^*} -\g^{j_2}_{\bm{\theta}_t^*} \right\|_2 \bigg\vert\mathcal{F}_t\right]\\
    &\leq \mathbb{E}\left[ \sum_{j=1}^M \left\| \Delta^{j}_{\bm{\theta}_t,\w_t^*} -\g^{j}_{\bm{\theta}_t^*} \right\|_2^2 + M\cdot\max_{k\in[M]}\left\| \Delta^{k}_{\bm{\theta}_t,\w_t^*} -\g^{k}_{\bm{\theta}_t^*} \right\|_2^2 \bigg\vert\mathcal{F}_t\right].
\end{align*}
\end{comment}

In addition, for any $j\in [M]$, we have
\begin{align*}
    &\hspace{13pt}\mathbb{E}\left[\left\|\Delta^{j}_{\bm{\theta}_t,\w_t^*} -\g^{j}_{\bm{\theta}_t^*}\right\|_2^2\bigg\vert\mathcal{F}_t\right]\\
    &= \mathbb{E}\left[\left\| \cfrac{1}{B}\sum_{l=0}^{B-1}\delta^j_{t,l}(\w^{j,*}_t)\cdot\bm{\psi}^{\bm{\theta}}_{t,l} - \Delta^j_{\bm{\theta}_t,\w_t^*}\right\|_2^2\bigg\vert\mathcal{F}_t\right]\\
    &= \mathbb{E}\left[ \left\langle \cfrac{1}{B}\sum_{l_1=0}^{B-1}\delta^j_{t,l_1}(\w^{j,*}_t)\cdot\bm{\psi}^{\bm{\theta}}_{t,l_1} - \Delta^j_{\bm{\theta}_t,\w_t^*}, \cfrac{1}{B}\sum_{l_2=0}^{B-1}\delta^j_{t,l_2}(\w^{j,*}_t)\cdot\bm{\psi}^{\bm{\theta}}_{t,l_2} - \Delta^j_{\bm{\theta}_t,\w_t^*} \right\rangle \bigg\vert\mathcal{F}_t\right]\\
    &= \mathbb{E}\left[ \cfrac{1}{B^2}\sum_{l=0}^{B-1}\left\|\delta^j_{t,l}(\w^{j,*}_t)\bm{\psi}^{\bm{\theta}}_{t,l} - \Delta^j_{\bm{\theta}_t,\w_t^*}\right\|_2^2 + \cfrac{1}{B^2}\sum_{l_1\neq l_2}\left\langle\delta^j_{t,l_1}(\w^{j,*}_t)\cdot\bm{\psi}^{\bm{\theta}}_{t,l_1} - \Delta^j_{\bm{\theta}_t,\w_t^*}, \delta^j_{t,l_2}(\w^{j,*}_t)\cdot\bm{\psi}^{\bm{\theta}}_{t,l_2} - \Delta^j_{\bm{\theta}_t,\w_t^*} \right\rangle \bigg\vert\mathcal{F}_t\right]\\
    &\overset{\text{(i)}}{\leq} \cfrac{16}{B}\left(r_{\max} +R_{\w}\right)^2 + \cfrac{1}{B^2}\sum_{l_1\neq l_2}\mathbb{E}\left[ \left\langle\delta^j_{t,l_1}(\w^{j,*}_t)\cdot\bm{\psi}^{\bm{\theta}}_{t,l_1} - \Delta^j_{\bm{\theta}_t,\w_t^*}, \delta^j_{t,l_2}(\w^{j,*}_t)\cdot\bm{\psi}^{\bm{\theta}}_{t,l_2} - \Delta^j_{\bm{\theta}_t,\w_t^*} \right\rangle \bigg\vert\mathcal{F}_t\right]\\
    &= \cfrac{16}{B}(r_{\max} +R_{\w})^2 + \cfrac{2}{B^2}\sum_{l_1<l_2}\mathbb{E}\left[ \left\langle\delta^j_{t,l_1}(\w^{j,*}_t)\cdot\bm{\psi}^{\bm{\theta}}_{t,l_1} - \Delta^j_{\bm{\theta}_t,\w_t^*}, \delta^j_{t,l_2}(\w^{j,*}_t)\cdot\bm{\psi}^{\bm{\theta}}_{t,l_2} - \Delta^j_{\bm{\theta}_t,\w_t^*} \right\rangle \bigg\vert\mathcal{F}_t\right]\\
    &= \cfrac{16}{B}(r_{\max} +R_{\w})^2 + \cfrac{2}{B^2}\sum_{l_1<l_2}\mathbb{E}\left[ \left\langle\delta^j_{t,l_1}(\w^{j,*}_t)\cdot\bm{\psi}^{\bm{\theta}}_{t,l_1} - \Delta^j_{\bm{\theta}_t,\w_t^*}, \mathbb{E}\left[\delta^j_{t,l_2}(\w^{j,*}_t)\cdot\bm{\psi}^{\bm{\theta}}_{t,l_2}\big\vert\mathcal{F}_{t,l_1}\right] - \Delta^j_{\bm{\theta}_t,\w_t^*} \right\rangle \bigg\vert\mathcal{F}_t\right]\\
    &\leq \cfrac{16}{B}(r_{\max} +R_{\w})^2 + \cfrac{2}{B^2}\sum_{l_1<l_2}\mathbb{E}\left[ \left\|\delta^j_{t,l_1}(\w^{j,*}_t)\cdot\bm{\psi}^{\bm{\theta}}_{t,l_1} - \Delta^j_{\bm{\theta}_t,\w_t^*}\right\|_2\cdot\left\|\mathbb{E}\left[\delta^j_{t,l_2}(\w^{j,*}_t)\cdot\bm{\psi}^{\bm{\theta}}_{t,l_2}\big\vert\mathcal{F}_{t,l_1}\right] - \Delta^j_{\bm{\theta}_t,\w_t^*}\right\|_2 \bigg\vert\mathcal{F}_t\right]\\
    &\leq \cfrac{16}{B}(r_{\max} +R_{\w})^2 + \cfrac{2}{B^2}\sum_{l_1<l_2}4\left(r_{\max}+R_{\w}\right)\mathbb{E}\left[\left\|\mathbb{E}\left[\delta^j_{t,l_2}(\w^{j,*}_t)\cdot\bm{\psi}^{\bm{\theta}}_{t,l_2}\big\vert\mathcal{F}_{t,l_1}\right] - \Delta^j_{\bm{\theta}_t,\w_t^*}\right\|_2 \bigg\vert\mathcal{F}_t\right]\\
    &\overset{\text{(ii)}}{\leq} \cfrac{16}{B}(r_{\max} +R_{\w})^2 + \cfrac{2}{B^2}\sum_{l_1<l_2}16(r_{\max} +R_{\w})^2\kappa\rho^{l_2-l_1},
\end{align*}
where (i) follows from the facts that
\begin{align*}
    |\delta^j_{t,l}(\w^{j,*}_t)|
    &= | r^{j}_{t,l+1}-\mu^{j}_{t,l}+\bm{\phi}(s_{t,l+1})^{\top}\w^{j}_t-\bm{\phi}(s_{t,l})^{\top}\w^{j}_t |_1\\
    &\leq | r^{j}_{t,l+1}|+|\mu^{j}_{t,l}|+\|\bm{\phi}(s_{t,l+1})-\bm{\phi}(s_{t,l})\|_2\cdot\|\w^{j}_t\|_2\\
    &\leq 2r_{\max} + 2R_{\w},
\end{align*}
thus, $\|\delta^j_{t,l}(\w^{j,*}_t)\bm{\psi}^{\bm{\theta}}_{t,l}\|_2\leq 2r_{\max} + 2R_{\w}$, and $\Delta^j_{\bm{\theta}_t, \w_t^*}=\mathbb{E}_{d_{\bm{\theta}}}\left[\mathbb{E}_{P_{\bm{\theta}}}\left[\delta_{t,l}^j(\w_t^{j,*})\mid(a_{t,l},s_{t,l})\right]\cdot\bm{\psi}^{\bm{\theta}}_{t, l}\right]\leq 2r_{\max} + 2R_{\w}$,
and (ii) follows from
\begin{align*}
    &\hspace{13pt}\left\|\mathbb{E}\left[\delta^j_{t,l_2}(\w^{j,*}_t)\cdot\bm{\psi}^{\bm{\theta}}_{t,l_2}\big\vert\mathcal{F}_{t,l_1}\right] - \Delta^j_{\bm{\theta}_t,\w_t^*}\right\|_2\\
    &= \left\|\mathbb{E}\left[\delta^j_{t,l_2}(\w^{j,*}_t)\cdot\bm{\psi}^{\bm{\theta}}_{t,l_2}\big\vert\mathcal{F}_{t,l_1}\right] - \mathbb{E}_{d_{\bm{\theta}}}\left[\mathbb{E}_{P_{\bm{\theta}}}\left[\delta_{t,l}^j(\w_t^{j,*})\mid(s_{t,l},a_{t,l})\right]\cdot\bm{\psi}^{\bm{\theta}}_{t, l}\right]\right\|_2\\
    &= \bigg\|\sum_{(s_{t,l_2},a_{t,l_2})}\mathbb{E}_{P_{\bm{\theta}}}\left[\delta_{t,l_2}^j(\w_t^{j,*})\mid(s_{t,l_2},a_{t,l_2})\right]\cdot\bm{\psi}^{\bm{\theta}}_{t, l}\cdot P(s_{t,l_2},a_{t,l_2}\mid\mathcal{F}_{t,l_1})\\
    &\hspace{13pt}-\sum_{(s_{t,l},a_{t,l})}\mathbb{E}_{P_{\bm{\theta}}}\left[\delta_{t,l}^j(\w_t^{j,*})\mid(s_{t,l},a_{t,l})\right]\cdot\bm{\psi}^{\bm{\theta}}_{t, l}\cdot\nu_{\bm{\theta}_t}(s_{t,l},a_{t,l}) \bigg\|_2\\
    &\leq \sum_{(s_{t,l},a_{t,l})}\left\| \mathbb{E}_{P_{\bm{\theta}}}\left[\delta_{t,l}^j(\w_t^{j,*})\mid(s_{t,l},a_{t,l})\right]\cdot\bm{\psi}^{\bm{\theta}}_{t, l} \right\|_2\cdot \left|P^{l_2-l_1}(s_{t,l},a_{t,l}\mid\mathcal{F}_{t,l_1})-\nu_{\bm{\theta}_t}(s_{t,l},a_{t,l})\right|\\
    &\overset{\text{(i)}}{\leq} 4(r_{\max} +R_{\w})\cdot\left\|P^{l_2-l_1}(s,a\mid\mathcal{F}_{t,l_1})-\nu_{\bm{\theta}_t}(s,a) \right\|_{TV}\\
    &\leq 4(r_{\max} +R_{\w})\kappa\rho^{l_2-l_1},
\end{align*}
where (i) follows from Lemma~\ref{lemma:tv2}.

Therefore, for the last term in Eq.~(\ref{eq:4}), we have
\begin{align}
    \mathbb{E}\left[ \left(\sum_{j=1}^M \lambda_t^j \cdot\left\| \Delta^j_{\bm{\theta}_t,\w_t^*} -\g^j_{\bm{\theta}_t^*}\right\|_2 \right)^2 \bigg\vert \mathcal{F}_t \right]
    &\leq \cfrac{16}{B}(r_{\max} +R_{\w})^2 + \cfrac{32}{B^2}\sum_{l_1<l_2}(r_{\max} +R_{\w})^2\kappa\rho^{l_2-l_1}\nonumber\\
    %&= \cfrac{32M}{B}(r_{\max} +R_{\w})^2 + \cfrac{32M}{B^2}(r_{\max} +R_{\w})^2\kappa\sum_{l_1<l_2}\rho^{l_2-l_1}\nonumber\\
    &\leq \cfrac{16}{B}(r_{\max} +R_{\w})^2 + \cfrac{32}{B^2}(r_{\max} +R_{\w})^2\cfrac{2\kappa\rho B}{1-\rho}\nonumber\\
    &= \cfrac{16(r_{\max} +R_{\w})^2(1-\rho+4\kappa\rho)}{(1-\rho)B}.\label{eq:7}
\end{align}
Substituting Eqs.~(\ref{eq:5}), (\ref{eq:6}), (\ref{eq:7}) into Eq.~(\ref{eq:4}) yields the expected gradient bias as follows
\begin{align}
    &\hspace{13pt}\mathbb{E}\left[\left\|\sum_{j=1}^M \lambda_t^j\left(\nabla_{\bm{\theta}}J^j(\bm{\theta}_t)-\g_t^j\right) \right\|^2_2\bigg\vert \mathcal{F}_t\right]\nonumber\\
    &\hspace{13pt} \le 12\zeta_{\text{approx}}+ 12\mathbb{E} \left[\left\| w^{i}_t-w^{i,*}_t\right\|^{2}_2 \bigg\vert  \mathcal{F}_t \right] + \cfrac{48(r_{\max} +R_{\w})^2(1-\rho+4\kappa\rho)}{(1-\rho)B}. \label{eq:8}
\end{align}
By letting $\alpha=\cfrac{1}{3L_J}$, we have
\begin{align}
\frac{2}{\alpha l_t-2\alpha^{2}l^{2}_t L_J}=\frac{18L_J}{-2l^{2}_t+3l_t}\le 16 L_J \nonumber
\end{align}
due to the facts $p_{\min}\le l_t\le 1$ and $p_{\min}\le \frac{1}{M}\le \frac{3}{4}=\arg\min_{l_t} -2l^{2}_t+3l_t$. Similarly, we also have
\begin{align}
\frac{\alpha+2\alpha^{2}l_t L_J}{\alpha-2\alpha^{2}l_tL_J}=\frac{3+2l_t}{3-2l_t}\le 5. \nonumber
\end{align}

Further, Substituting Eq.~(\ref{eq:8}) into Eq.~(\ref{eq: dir_mod}) and taking expectation of $\mathcal{F}_t$ yield
\begin{align}
    \mathbb{E}\left[ \left\|\nabla_{\bm{\theta}}\bm{J}(\bm{\theta}_t)\bm{\lambda}_t^*\right\|^2_2 \right]
    &\leq 16L_J\left(\mathbb{E}\left[\bm{q}_t^\top\bm{J}(\bm{\theta}_{t+1})\right] - \bm{q}_t^\top\bm{J}(\bm{\theta}_t)\right) + 60{\zeta_{\text{approx}}} + 60\max_{j\in [M]}\mathbb{E}\left[\left\|\w^j_t - \w^{j,*}_t\right\|_2^2\right]\nonumber\\
    &\hspace{13pt}+ \cfrac{240(r_{\max} +R_{\w})^2(1-\rho+4\kappa\rho)}{(1-\rho)B}.
\label{eq:9}
\end{align}
% \begin{align}
%     &\hspace{13pt}\mathbb{E}\left[ \left\|\nabla_{\bm{\theta}}\bm{J}(\bm{\theta}_t)\bm{\lambda}_t^*\right\|^2_2 \right]\nonumber\\
%     &\leq \cfrac{2\left(\mathbb{E}\left[\bm{\lambda}_t^\top\bm{J}(\bm{\theta}_{t+1})\vert \mathcal{F}_t\right] - \bm{\lambda}_t^\top\bm{J}(\bm{\theta}_t)\right)}{\alpha-2\alpha^2L_J}\nonumber\\
%     &\hspace{13pt}+ \cfrac{\alpha+2\alpha^2L_J}{\alpha-2\alpha^2L_J}\left[ 8M^2{\zeta_{\text{approx}}(t)} + 8M^2\mathbb{E}\left[\left\|\w^j_t - \w^{j,*}_t\right\|_2^2\right]+ \cfrac{32M(r_{\max} +R_{\w})^2(1-\rho+2\kappa\rho)}{(1-\rho)B} \right]\nonumber\\
%     &= 18L_J\left(\mathbb{E}\left[\bm{\lambda}_t^\top\bm{J}(\bm{\theta}_{t+1})\vert \mathcal{F}_t\right] - \bm{\lambda}_t^\top\bm{J}(\bm{\theta}_t)\right) + 40M^2{\zeta_{\text{approx}}(t)} + 40M^2\mathbb{E}\left[\left\|\w^j_t - \w^{j,*}_t\right\|_2^2\right]\nonumber\\
%     &\hspace{13pt}+ \cfrac{160M(r_{\max} +R_{\w})^2(1-\rho+2\kappa\rho)}{(1-\rho)B}.\label{eq:9}
% \end{align}

\subsection{For the 1st Term on RHS of Eq.~\eqref{eq: dir_mod}}
Let $\hat{T}$ denote a random variable that takes value uniformly random among $\lbrace 1, \ldots, T\rbrace$, then taking average of Eq.~(\ref{eq:9}) over $T$ and we have
\begin{align*}
    \mathbb{E}\left[ \left\|\nabla_{\bm{\theta}}\bm{J}(\bm{\theta}_{\hat{T}})\bm{\lambda}_{\hat{T}}^*\right\|^2_2 \right]
    &= \cfrac{1}{T}\sum_{t=1}^T\mathbb{E}\left[ \left\|\nabla_{\bm{\theta}}\bm{J}(\bm{\theta}_t)\bm{\lambda}_t^*\right\|^2_2 \right]\\
    &\leq \cfrac{16L_J}{T}\sum_{t=1}^T\left(\mathbb{E}\left[\bm{q}_t^\top\bm{J}(\bm{\theta}_{t+1})\right] - \bm{q}_t^\top\bm{J}(\bm{\theta}_t)\right) + \cfrac{60}{T}\sum_{t=1}^T\max_{j\in [M]}\mathbb{E}\left[\left\|\w^j_t - \w^{j,*}_t\right\|_2^2\right]\\
    &\hspace{13pt}+ \cfrac{240(r_{\max} +R_{\w})^2(1-\rho+4\kappa\rho)}{(1-\rho)B} + 60\zeta_{\text{approx}}.
\end{align*}
Specifically,
\begin{align*}
    \sum_{t=1}^T\left(\mathbb{E}\left[\bm{q}_t^\top\bm{J}(\bm{\theta}_{t+1})\right] - \bm{q}_t^\top\bm{J}(\bm{\theta}_t)\right)
    &= \mathbb{E}\left[ \sum_{t=1}^{T-1}(-\bm{q}_{t+1}+\bm{q}_t)^\top\bm{J}(\bm{\theta}_{t+1}) - \bm{q}^\top_1\bm{J}(\bm{\theta}_1) + \bm{q}^\top_T\bm{J}(\bm{\theta}_{T+1}) \right]\\
    &\overset{\text{(i)}}{\leq} \mathbb{E}\left[ \sum_{t=1}^{T-1}|\bm{q}_{t+1}-\bm{q}_t|_{1} \|\bm{J}(\bm{\theta}_{t+1})\|_{\infty} + \|\bm{q}_T\|_{1}\|\bm{J}(\bm{\theta}_{T+1})\|_{\infty} \right]\\
    &\leq r_{\max} + r_{\max}\sum_{t=1}^{T} \mathbb{E}\left[|\bm{q}_{t+1}-\bm{q}_t|_{1}\right]\\
    &\leq r_{\max} \left(1+ \frac{2}{p_{\min}}\sum_{t=1}^{T}\eta_t\right),
\end{align*}
where (i) follows from H\"older's Inequality since $1/1+1/\infty=1$. Meanwhile, the above result also used the facts
\begin{align}
\bm{q}_{t+1}-\bm{q}_t &= \frac{\bm{\lambda}_{t+1}\odot \p}{l_{t+1}}-\frac{\bm{\lambda}_t\odot \p}{l_t} \nonumber \\
& = \left(\frac{\bm{\lambda}_{t+1}}{l_{t+1}}-\frac{\bm{\lambda}_t}{l_t} \right)\odot \p \nonumber
\end{align}
and
\begin{align}
\frac{\bm{\lambda}_{t+1}}{l_{t+1}}-\frac{\bm{\lambda}_t}{l_t} &= \frac{(1-\eta_t)\bm{\lambda}_t+\eta_t \hat{\bm{\lambda}}^*_t}{l_{t+1}}-\frac{\bm{\lambda}_t}{l_t} \nonumber \\
&=\frac{\left[(1-\eta_t)\bm{\lambda}_t+\eta_t \hat{\bm{\lambda}}^*_t\right]\langle \bm{\lambda}_t,\p \rangle-(1-\eta_t)\bm{\lambda}_t\langle \bm{\lambda}_t,\p\rangle-\eta_t\bm{\lambda}_t\langle \hat{\bm{\lambda}}^*_t,\p\rangle}{l_{t+1}l_t} \nonumber \\
&=\frac{\eta_t\left(\hat{\bm{\lambda}}^*_t\langle \bm{\lambda}_t,\p \rangle-\bm{\lambda}_t\langle \hat{\bm{\lambda}}^*_t,\p\rangle\right)}{l_{t+1}l_t}. \nonumber 
\end{align}
By the above, we have
\begin{align}
\left| \bm{q}_{t+1}-\bm{q}_t \right|_1 &\le \left|\frac{\eta_t\left(\hat{\bm{\lambda}}^*_t\langle \bm{\lambda}_t,\p \rangle-\bm{\lambda}_t\langle \hat{\bm{\lambda}}^*_t,\p\rangle\right)}{l_{t+1}l_t}\right|_1 \nonumber \\
& \le \frac{\eta_t}{p^{2}_{\min}}(\left|\hat{\bm{\lambda}}^*_t\langle \bm{\lambda}_t,\p \rangle\right|_1+\left|\bm{\lambda}_t\langle \hat{\bm{\lambda}}^*_t,\p\rangle\right|) \nonumber \\
& \le \frac{2\eta_t}{p^{2}_{\min}}. \label{eq: q_bound}
\end{align}
This facilitates the analysis to be $M$-independent in the telescoping process.
Then, we have
\begin{align*}
    \mathbb{E}\left[ \left\|\nabla_{\bm{\theta}}\bm{J}(\bm{\theta}_{\hat{T}})\bm{\lambda}^{*}_{\hat{T}}\right\|^2_2 \right]
    &\leq \cfrac{16L_J r_{\max}}{T}\left(1 + \frac{2}{p^{2}_{\min}}\sum_{t=1}^T\eta_t \right)+\cfrac{60}{T}\sum_{t=1}^T\max_{j\in [M]}\mathbb{E}\left[\left\|\w^j_t - \w^{j,*}_t\right\|_2^2\right]\\
    &\hspace{13pt}+ \cfrac{240(r_{\max} +R_{\w})^2(1-\rho+4\kappa\rho)}{(1-\rho)B} + 60\zeta_{\text{approx}}.
\end{align*}

\subsection{Final Result for Average Reward Setting}
Recalling that $\alpha=\cfrac{1}{3L_J}$ and by letting $T\geq \cfrac{48L_J r_{\max}}{\epsilon}\cdot(1+\frac{2}{p^{2}_{\min}}\sum_{t=1}^T\eta_t)$, $\mathbb{E}\left[\left\|\w^j_t - \w^{j,*}_t\right\|_2^2\right]\leq \cfrac{\epsilon}{180}$ for any objective $j\in[M]$, and $B\geq \cfrac{720(r_{\max} +R_{\w})^2(1-\rho+4\kappa\rho)}{\epsilon}$ yields
\begin{equation*}
    \mathbb{E}\left[ \left\|\bm{\lambda}_{\hat{T}}^\top\nabla_{\bm{\theta}}\bm{J}(\bm{\theta}_{\hat{T}})\right\|^2_2 \right] \leq \epsilon + 60\zeta_{\text{approx}},
\end{equation*}
with a total sample complexity given by
\begin{equation*}
    (B+ND)T=\mathcal{O}\left( \left(\cfrac{1}{\epsilon}+\cfrac{1}{\epsilon}\log\cfrac{1}{\epsilon}\right)\cfrac{1}{\epsilon p^{2}_{\min}} \right) = \mathcal{O}\left(\cfrac{1}{\epsilon^2 p^{2}_{\min}}\log\cfrac{1}{\epsilon}\right).
\end{equation*}

\subsection{Final Result for Discounted Reward Setting}
Similar to the proof in average reward setting, we have
\begin{equation}
    \mathbb{E}\left[ \left\|\nabla_{\bm{\theta}}\bm{J}(\bm{\theta}_t)\bm{\lambda}_t^*\right\|^2_2 \mid \mathcal{F}_t \right] \leq \cfrac{2\left(\mathbb{E}\left[\bm{\lambda}_t^\top\bm{J}(\bm{\theta}_{t+1})\vert \mathcal{F}_t\right] - \bm{\lambda}_t^\top\bm{J}(\bm{\theta}_t)\right)}{\alpha-2\alpha^2L_J} + \cfrac{\alpha+2\alpha^2L_J}{\alpha-2\alpha^2L_J}\mathbb{E}\left[\left\|\sum_{j=1}^M \lambda_t^j\left(\nabla_{\bm{\theta}}J^j(\bm{\theta}_t)-\g_t^j\right) \right\|^2_2\bigg\vert \mathcal{F}_t\right],
\label{eq:10}
\end{equation}
where the last term on the right hand side is bounded by
\begin{align}
&\hspace{13pt}\mathbb{E}\left[\left\|\sum_{j=1}^M \lambda_t^j\left(\nabla_{\bm{\theta}}J^j(\bm{\theta}_t)-\g_t^j\right) \right\|^2_2\bigg\vert \mathcal{F}_t\right] \nonumber\\
 &\le 3\mathbb{E}\left[\left(\sum_{j=1}^M \lambda_t^j \left\| \nabla_{\bm{\theta}}J^j(\bm{\theta}_t) - \Delta^j_{\bm{\theta}_t,\w_t^*}\right\|_2  \right)^2\bigg\vert \mathcal{F}_t \right] \nonumber \\
 &\hspace{13pt}+3\mathbb{E}\left[\left(\sum_{j=1}^M \lambda_t^j \left\| \g^j_{\bm{\theta}_t^*} - \g_t^j\right\|_2 \right)^{2}\bigg\vert  \mathcal{F}_t \right] + 3\mathbb{E}\left[ \left(\sum_{j=1}^M \lambda_t^j \cdot\left\| \Delta^j_{\bm{\theta}_t,\w_t^*} -\g^j_{\bm{\theta}_t^*}\right\|_2 \right)^2 \bigg\vert \mathcal{F}_t \right].
%&\leq \mathbb{E}\left[ \left|\sum_{j=1}^M \lambda_t^j \left(\left\| \nabla_{\bm{\theta}}J^j(\bm{\theta}_t) - \Delta^j_{\bm{\theta}_t,\w_t^*}\right\|_2 + \left\| \g^j_{\bm{\theta}_t^*} - \g_t^j\right\|_2 \right) \right|^2 \bigg\vert \mathcal{F}_t \right]\nonumber\\
%&\hspace{13pt}+ \mathbb{E}\left[ \left|\sum_{j=1}^M \lambda_t^j \cdot\left\| \Delta^j_{\bm{\theta}_t,\w_t^*} -\g^j_{\bm{\theta}_t^*}\right\|_2 \right|^2 \bigg\vert \mathcal{F}_t \right].
\label{eq:11}
\end{align}
Considering the discounted factor $\gamma$, we have
\begin{equation}
    \left\| \nabla_{\bm{\theta}}J^j(\bm{\theta}_t) - \Delta^j_{\bm{\theta}_t,\w_t^*}\right\|_2 \leq 2\sqrt{\zeta_{\text{approx}}},
\label{eq:12}
\end{equation}
and
\begin{equation}
    \left\| \g^j_{\bm{\theta}_t^*} - \g_t^j\right\|_2\leq 2\cdot\left\| \w^j_t - \w^{j,*}_t \right\|_2.
\label{eq:13}
\end{equation}
For the last term in Eq.~(\ref{eq:11}), we have
\begin{equation}
    \mathbb{E}\left[ \left|\sum_{j=1}^M \lambda_t^j \cdot\left\| \Delta^j_{\bm{\theta}_t,\w_t^*} -\g^j_{\bm{\theta}_t^*}\right\|_2 \right|^2 \bigg\vert \mathcal{F}_t \right] \leq \cfrac{4(r_{\max} +2R_{\w})^2(1-\rho+4\kappa\rho)}{(1-\rho)B},
\label{eq:14}
\end{equation}
since the facts
\begin{align*}
    |\delta^j_{t,l}(\w^{j,*}_t)|
    &= | r^{j}_{t,l+1}+\gamma\bm{\phi}(s_{t,l+1})^{\top}\w^{j}_t-\bm{\phi}(s_{t,l})^{\top}\w^{j}_t |_1\\
    &\leq | r^{j}_{t,l+1}|+\|\gamma\bm{\phi}(s_{t,l+1})-\bm{\phi}(s_{t,l})\|_2\cdot\|\w^{j}_t\|_2\\
    &\leq r_{\max} + 2R_{\w},
\end{align*}
thus, $\|\delta^j_{t,l}(\w^{j,*}_t)\bm{\psi}^{\bm{\theta}}_{t,l}\|_2\leq r_{\max} + 2R_{\w}$, and $\Delta^j_{\bm{\theta}_t, \w_t^*}=\mathbb{E}_{d_{\bm{\theta}}}\left[\mathbb{E}_{P_{\bm{\theta}}}\left[\delta_{t,l}^j(\w_t^{j,*})\mid(a_{t,l},s_{t,l})\right]\cdot\bm{\psi}^{\bm{\theta}}_{t, l}\right]\leq r_{\max} + 2R_{\w}$.

Substituting Eqs.~(\ref{eq:12}), (\ref{eq:13}), (\ref{eq:14}) into Eq.~(\ref{eq:11}), we have
\begin{equation}
    \mathbb{E}\left[\left\|\sum_{j=1}^M \lambda_t^j\left(\nabla_{\bm{\theta}}J^j(\bm{\theta}_t)-\g_t^j\right) \right\|^2_2\bigg\vert \mathcal{F}_t\right] \leq 12{\zeta_{\text{approx}}} + 12\max_{j\in[M]}\mathbb{E}\left[\left\|\w^j_t - \w^{j,*}_t\right\|_2^2 \bigg\vert\mathcal{F}_t\right] + \cfrac{12(r_{\max} +2R_{\w})^2(1-\rho+4\kappa\rho)}{(1-\rho)B}.
\label{eq:15}
\end{equation}

Substituting Eq.~(\ref{eq:15}) into Eq.~(\ref{eq:10}), letting $\alpha=\cfrac{1}{3L_J}$, taking expectation of $\mathcal{F}_t$, and taking average of Eq.~(\ref{eq:10}) over $T$ yields
\begin{align*}
    \mathbb{E}\left[ \left\|\nabla_{\bm{\theta}}\bm{J}(\bm{\theta}_{\hat{T}})\bm{\lambda}_{\hat{T}}^*\right\|^2_2 \right]
    &= \cfrac{1}{T}\sum_{t=1}^T\mathbb{E}\left[ \left\|\nabla_{\bm{\theta}}\bm{J}(\bm{\theta}_t)\bm{\lambda}_t^*\right\|^2_2 \right]\\
    &\leq \cfrac{16L_J}{T}\sum_{t=1}^T\left(\mathbb{E}\left[\bm{\lambda}_t^\top\bm{J}(\bm{\theta}_{t+1})\right] - \bm{\lambda}_t^\top\bm{J}(\bm{\theta}_t)\right) + \cfrac{60}{T}\sum_{t=1}^T\max_{j\in[M]}\mathbb{E}\left[\left\|\w^j_t - \w^{j,*}_t\right\|_2^2\right]\\
    &\hspace{13pt}+ \cfrac{60(r_{\max} +2R_{\w})^2(1-\rho+4\kappa\rho)}{(1-\rho)B} + 60\zeta_{\text{approx}},
\end{align*}
where
\begin{align*}
    \sum_{t=1}^T\left(\mathbb{E}\left[\bm{q}_t^\top\bm{J}(\bm{\theta}_{t+1})\right] - \bm{q}_t^\top\bm{J}(\bm{\theta}_t)\right)
    &= \mathbb{E}\left[ \sum_{t=1}^{T-1}(-\bm{q}_{t+1}+\bm{q}_t)^{\top}\bm{J}(\bm{\theta}_{t+1}) - \bm{q}^{\top}_1\bm{J}(\bm{\theta}_1) + \bm{q}^{\top}_T\bm{J}(\bm{\theta}_{T+1}) \right]\\
    &\leq \mathbb{E}\left[ \sum_{t=1}^{T-1}|\bm{q}_{t+1}-\bm{q}_t|_1 \|\bm{J}(\bm{\theta}_{t+1})\|_{\infty} + |\bm{q}_T|_1\|\bm{J}(\bm{\theta}_{T+1})\|_{\infty} \right]\\
    &\leq \sum_{t=1}^{T-1} \left(\frac{2\eta_t}{p^{2}_{\min}}\cdot\frac{r_{\max}}{1-\|\bm{\gamma}\|_\infty}\right) + \cfrac{r_{\max}}{1-\|\bm{\gamma}\|_\infty}\\
    &\leq \cfrac{r_{\max}}{1-\|\bm{\gamma}\|_\infty}(1+\frac{2}{p^{2}_{\min}}\sum_{t=1}^{T}\eta_t),
\end{align*}
where the 2nd from the last inequality, we used inequality \ref{eq: q_bound} for discounted setting.
Then, we have
\begin{align*}
    \mathbb{E}\left[ \left\|\nabla_{\bm{\theta}}\bm{J}(\bm{\theta}_{\hat{T}})\bm{\lambda}_{\hat{T}}\right\|^2_2 \right]
    &\leq \cfrac{16L_J r_{\max}}{T(1-\|\bm{\gamma}\|_\infty)}(1+\frac{2}{p^{2}_{\min}}\sum_{t=1}^{T}\eta_t)+ \cfrac{60}{T}\sum_{t=1}^T\max_{j\in[M]}\mathbb{E}\left[\left\|\w^j_t - \w^{j,*}_t\right\|_2^2\right]\\
    &\hspace{13pt}+ \cfrac{60(r_{\max} +2R_{\w})^2(1-\rho+4\kappa\rho)}{(1-\rho)B} + 60\zeta_{\text{approx}}.
\end{align*}
By letting $T\geq \cfrac{48L_J r_{\max}}{\epsilon(1-\|\bm{\gamma}\|_\infty)}\cdot (1+ \frac{2}{p^{2}_{\min}}\sum_{t=1}^T\eta_t)$, $\mathbb{E}\left[\left\|\w^j_t - \w^{j,*}_t\right\|_2^2\right]\leq \cfrac{\epsilon}{240}$ for any objective $j\in[M]$, and $B\geq \cfrac{240(r_{\max} +2R_{\w})^2(1-\rho+4\kappa\rho)}{\epsilon}$ yields
\begin{equation*}
    \mathbb{E}\left[ \left\|\bm{\lambda}_{\hat{T}}^\top\nabla_{\bm{\theta}}\bm{J}(\bm{\theta}_{\hat{T}})\right\|^2_2 \right] \leq \epsilon + 60\zeta_{\text{approx}},
\end{equation*}
with total sample complexity given by
\begin{equation*}
    (B+ND)T=\mathcal{O}\left( \left(\cfrac{1}{\epsilon}+\cfrac{1}{\epsilon}\log\cfrac{1}{\epsilon}\right)\cfrac{1}{\epsilon p^{2}_{\min}} \right) = \mathcal{O}\left(\cfrac{1}{\epsilon^2 p^{2}_{\min}}\log\cfrac{1}{\epsilon}\right).
\end{equation*}
\end{proof}
